# Supplementary material for: TrAct: Bridging Robot Control and Visual Prediction with Visual Tracks
Source: arXiv:2608.24101 source file (2026-10-13)
Supplement: Supplementary file 1 [file appendix-main.tex]

\documentclass{article}

\usepackage{corl_2026} % Use this for the initial submission.
% \usepackage[final]{corl_2026} % Uncomment for the camera-ready ``final'' version.
% \usepackage[preprint]{corl_2026} % Uncomment for pre-prints (e.g., arxiv); This is like ``final'', but will remove the CORL footnote.
\usepackage{multirow}
\usepackage{booktabs}
\usepackage{tabularx}
\usepackage{array}
\usepackage{graphicx}
\usepackage{amsmath}
\usepackage{amssymb}
\usepackage{bm}
\usepackage{xspace}
\usepackage{algorithm}
\usepackage{algpseudocode}

%\usepackage{xcolor}

\newcommand{\todo}[1]{\textcolor{red}{[#1]}}
\newcommand{\algabbr}{TrAct\xspace}

\title{TrAct: Bridging Robot Control and Visual Prediction with Visual Tracks}

% The \author macro works with any number of authors. There are two
% commands used to separate the names and addresses of multiple
% authors: \And and \AND.
%
% Using \And between authors leaves it to LaTeX to determine where to
% break the lines. Using \AND forces a line break at that point. So,
% if LaTeX puts 3 of 4 authors names on the first line, and the last
% on the second line, try using \AND instead of \And before the third
% author name.

% NOTE: authors will be visible only in the camera-ready and preprint versions (i.e., when using the option 'final' or 'preprint'). 
% 	For the initial submission the authors will be anonymized.

\author{
  Jane E.~Doe\\
  Department of Electrical Engineering and Computer Sciences\\
  University of California Berkeley 
  United States\\
  \texttt{janedoe@berkeley.edu} \\
  %% examples of more authors
  %% \And
  %% Coauthor \\
  %% Affiliation \\
  %% Address \\
  %% \texttt{email} \\
  %% \AND
  %% Coauthor \\
  %% Affiliation \\
  %% Address \\
  %% \texttt{email} \\
  %% \And
  %% Coauthor \\
  %% Affiliation \\
  %% Address \\
  %% \texttt{email} \\
  %% \And
  %% Coauthor \\
  %% Affiliation \\
  %% Address \\
  %% \texttt{email} \\
}


\begin{document}

%===============================================================================

% no \bibliographystyle is required, since the corl style is automatically used.

\clearpage
\appendix
\input{sections/appendix}
\clearpage
\bibliography{example}  % .bib

\end{document}
